# Supplementary material for: Chemical Potential Calculations In Dense Liquids Using Metadynamics
Source: arXiv:1604.07565 ancillary file (2016-07-25)
Supplement: Supplementary file 1 [file SI2arx.pdf]

Supporting Information for: Chemical Potential Calculations In Dense Liquids Using Metadynamics

C. Perego,[1,2] F. Giberti,[3] and M. Parrinello[1,2,a)]
1) *Department of Chemistry and Applied Biosciences, ETH Zurich, Zurich (Switzerland)*
2) *Institute of Computational Science, Università della Svizzera italiana, Lugano (Switzerland)*
3) *Institute for Molecular Engineering, The University of Chicago, Chicago (United States)*

## I. NUMBER OF SAMPLING POINTS

We studied the dependence of the convergence of $\mu_\alpha^{\text{ex}}$ with the number of insertion points $M$. In Fig. 1 it can be seen that, with the exception of the $M = 1$ case, whose convergence is very slow, all calculations converge to the same result.

Not surprisingly, the larger $M$, the smaller the error, but even with a relatively small number of points ($M = 2 \times 2 \times 2$) a satisfactory accuracy is attained. The use of a large $M$ is less convenient in terms of computational load and one should tune $M$ according to the considered system and computational resources. In our hand the best compromise seemed to be the $M = 4 \times 4 \times 4$ case. With this choice the distance between the closest $\mathbf{R}_i^*$'s ($d = 2.17$) is slightly larger than the correlation length of the fluid ($\lambda \sim 2$).

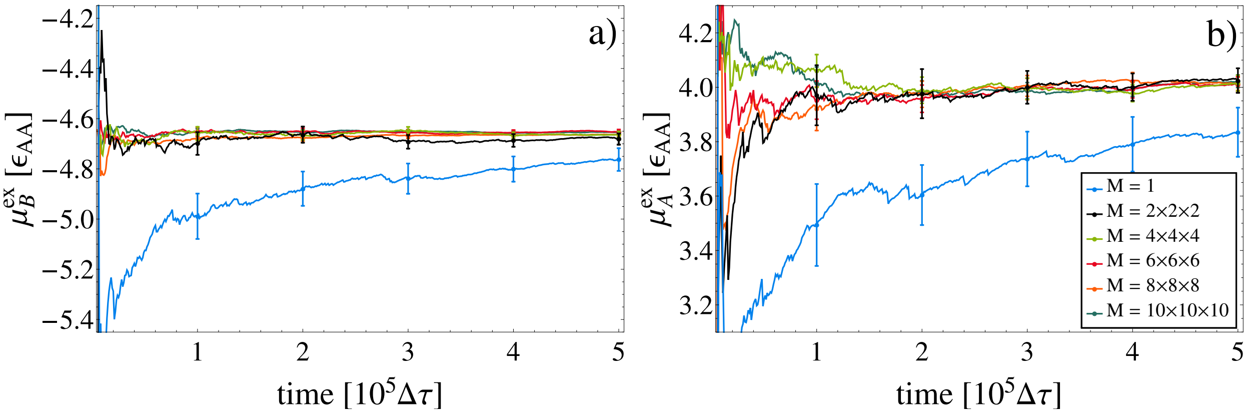


FIG. 1. Estimate of $\mu_\alpha^{\text{ex}}$ for different values of $M$. $\mu_B^{\text{ex}}$ is reported in panel a and $\mu_A^{\text{ex}}$ in panel b. As shown in the legend (valid for both panels) different colors correspond to different $M$'s. The error bars are computed combining block average and bootstrap methods[1].

## II. $F(s)$ AND $\mu^{\text{ex}}$

In this section we show the relevance of the different regions of the $s_\alpha$ space for the computation of $\mu_\alpha^{\text{ex}}$. According to Eq. (22) of the main text we can compute $\mu_\alpha^{\text{ex}}$ by integrating the free energy over $s_\alpha$. Beacuse of the term $\exp(-\beta s_\alpha)$ at the numerator of Eq. (22) it follows that the small $s_\alpha$ configurations contribute the most to $\mu_\alpha^{\text{ex}}$.

We show this by calculating the following function:

$$z_\alpha(\bar{s}_\alpha) = \frac{\int_{\bar{s}_\alpha}^{\infty} \mathrm{e}^{-\beta[F(s_\alpha)+s_\alpha]} \mathrm{d}s_\alpha}{\int_{\bar{s}_\alpha}^{\infty} \mathrm{e}^{-\beta F(s_\alpha)} \mathrm{d}s_\alpha}, \tag{1}$$

which is related to the chemical potential by the limit:

$$\lim_{\bar{s}_\alpha \to -\infty} z_\alpha(\bar{s}_\alpha) = \mathrm{e}^{-\beta \mu_\alpha^{\text{ex}}} \tag{2}$$

a) Electronic mail: michele.parrinello@phys.chem.ethz.ch

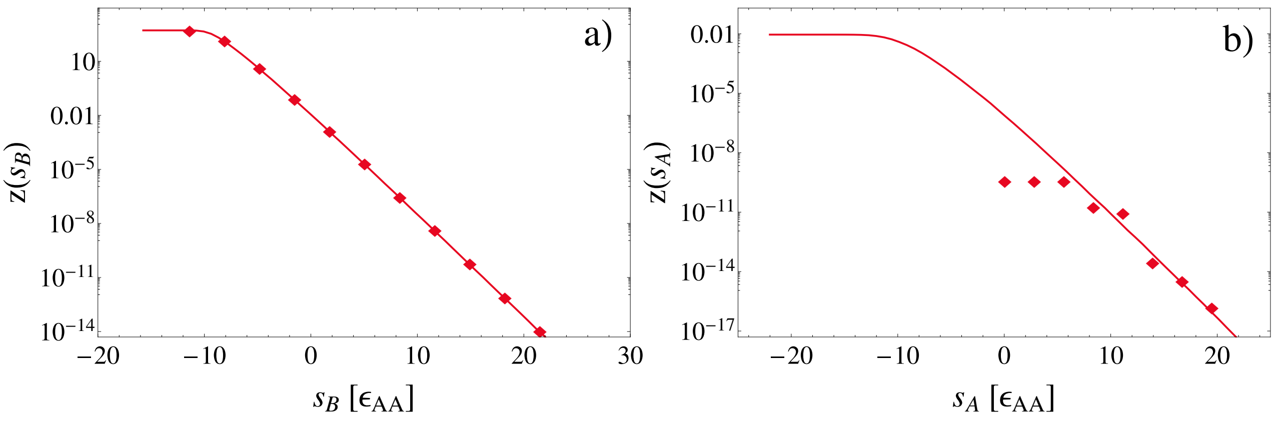


FIG. 2. Plot of $z(s_\alpha)$ function for $\alpha = B$ (panel a) and $\alpha = A$ (panel b). The red line represents the metadynamics result while the diamonds represent the unbiased result. The plot is obtained from the free energies displayed in Figure 1 of the main text, the simulation parameters are reported there.

In Fig. 2 we plot $z_\alpha$ for both the unbiased and metadynamics simulations. It is clear that, in the $\alpha = A$ case, the limit in Eq. (2) can be reached only using metadynamics.

## III. REGULARIZED CV DISTRIBUTION

In this section we show that the regularized variable $s^{\mathrm{r}}_\alpha$ has the same distribution of $s_\alpha$ in the region which contributes to the chemical potential calculation. This is shown in Fig. 3 where the free energy surface $F(s^{\mathrm{r}}_\alpha)$ is compared to the corresponding $F(s_\alpha)$. The difference in the two free energy profiles becomes relevant only for $s_\alpha \gtrsim 10$, a region which yields a negligible contribution to the chemical potential (see Sec. II). As a result $\mu^{\mathrm{ex}}_\alpha$ can be estimated either using the distribution of $s^{\mathrm{r}}_\alpha$ or reweigthing it to obtain the distribution of $s_\alpha$. In both cases we obtain identical results (see Fig. 4).

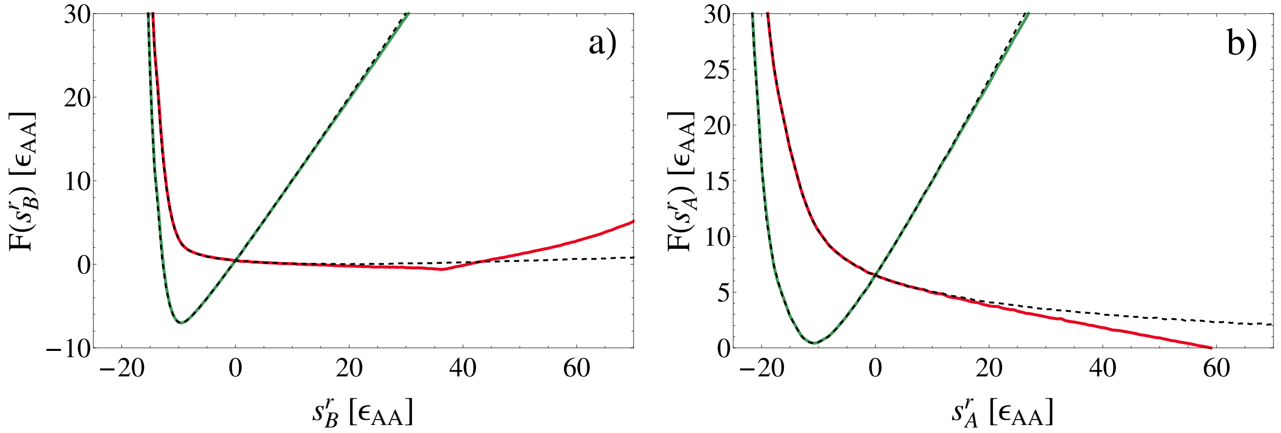


FIG. 3. Plot of $F(s^{\mathrm{r}}_\alpha)$ (red) and $F(s^{\mathrm{r}}_\alpha) + s^{\mathrm{r}}_\alpha$ (green) for $\alpha = B$ (panel a) and $\alpha = A$ (panel b). The dashed black lines represent $F(s_\alpha)$ and $F(s_\alpha) + s_\alpha$. We refer to Figure 1 of the main text for the simulation parameters.

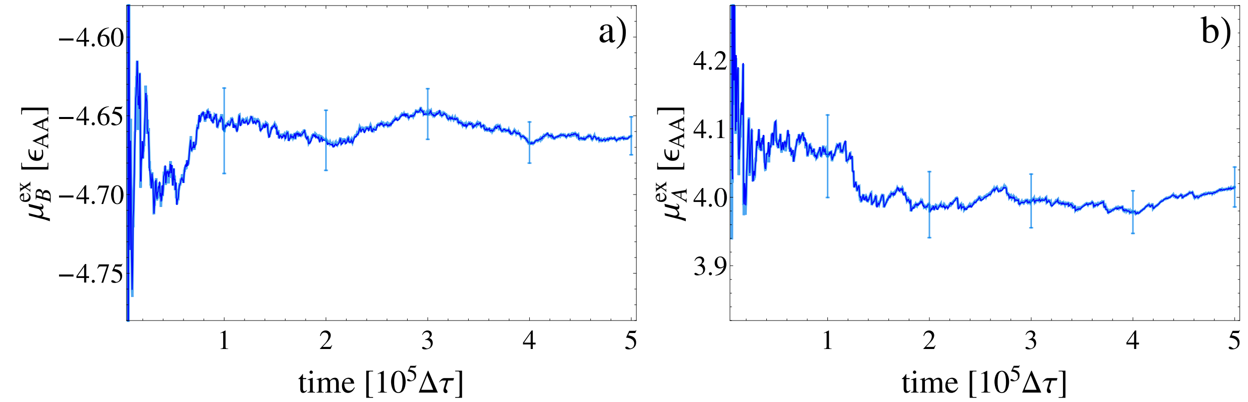


FIG. 4. $\mu_\alpha^{ex}$ computed averaging over $s_\alpha^r$ sampling (light blue thick line) and $s_\alpha$ sampling (blue thin line). $\mu_B^{ex}$ is reported in panel a and $\mu_A^{ex}$ in panel b, in both panels the two curves overlap. The error bars are computed combining block average and bootstrap methods[1].

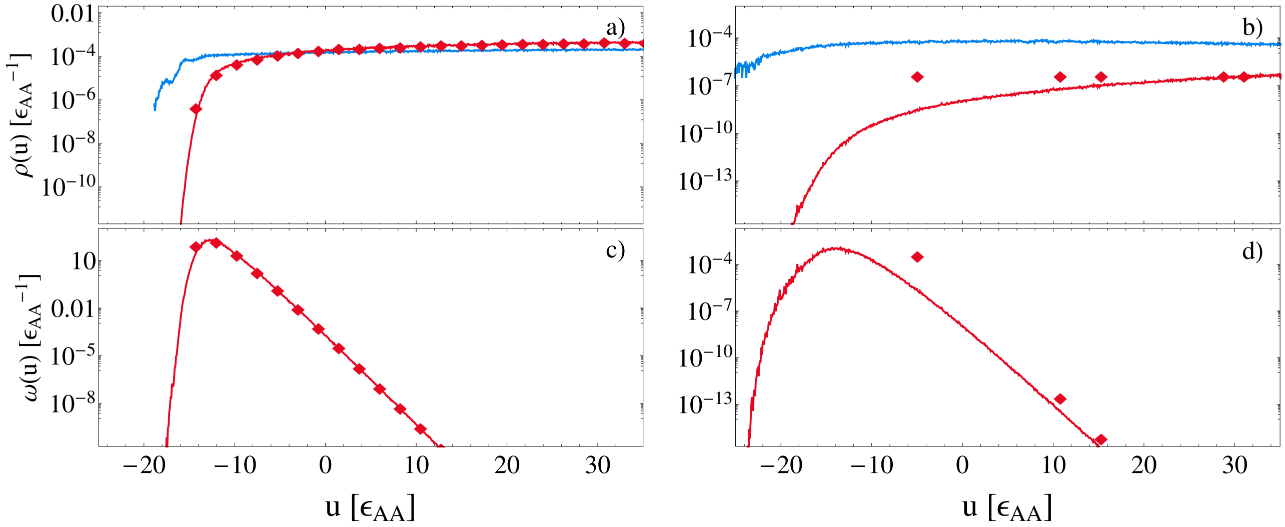


FIG. 5. Probability distribution of insertion energies $\rho(u)$ obtained from metadynamics calculations biasing $s_B$ (panel a), and $s_A$ (panel b). The blue lines represent the sampled biased distributions while the red lines are the reweighted results. In the lower panels the function $w(u) = \rho(u)\exp(-\beta u)$ is plotted for $\alpha = B$ (panel c) and $\alpha = A$ (panel d). In all four panels the diamonds indicate the distributions sampled with Widom's method. In both Widom's and metadynamics calculations $M = 64$ insertions per $\Delta\tau$ were computed. All the distributions are obtained from $5 \times 10^5\ \Delta\tau$ long runs.

## IV. INSERTION ENERGY DISTRIBUTIONS

In this section we report the probability density of the insertion energy $\Delta U_\alpha(\mathbf{R}_i^*; \mathbf{R})$, given by the canonical average

$$\rho(u) = \left\langle \frac{1}{M} \sum_{i=1}^{M} \delta[u - \Delta U_\alpha(\mathbf{R}_i^*; \mathbf{R})] \right\rangle . \tag{3}$$

In Fig. 5 we compare the $\rho(u)$ sampled with metadynamics to that resulting from ordinary Widom method. The comparison shows how our method allows to reconstruct the relevant negative tail of the insertion energy, which is not accessible using unbiased insertions.

[1]H. Flyvbjerg, H. G. Petersen, J. Chem. Phys. **91**(1), (1989) 461
